# Supplementary material for: Block-Skim: Efficient Question Answering for Transformer
Source: arXiv:2112.08560 source file (2022-05-15)
Supplement: Supplementary file 2 [file probing.tex]

\section{Probing Experiment Setting} \label{sec:probing}

As demonstrated in \Sec{sec:background}, we use a probing experiment to evaluate whether attention weights is informative for skimming prediction.
In this section, we give a detailed explanation of the experiment settings.

% To answer the above question, we build a simple logistic regression model with attention weights to predict whether an input sentence block contains the answer.
% To answer the above question, we build a simple logistic regression model with attention matrix from each layer to predict whether an input sentence block contains the answer.
% A block is defined as a continuos region in the input sequence from some position i to j.
% Given a input sequence, a block is a continuos region from position i to j as shown in \Fig{fig:posthoc}.
Given a input sequence, we split it to several continuos blocks with a fixed block size as hyper-parameter.
We are not partitioning the sequence with some linguistic boundaries for the convenience of aligned computation.
Our experiment results show that this split manner doesn't reduce any accuracy.

% This probing experiment is able to evaluate  whether the attention weights are informative enough on identifying the answer region.
% The attention weights of a block is flattened as the feature vector for classification.\footnote{The detailed setting for the classification feature and logistic regression is demonstrated in \Sec{sec:logistic_regression} }
% The attention matrices are profiled from a \model{BERT}{large} SQuAD QA model.
The attention matrices are profiled from a \model{BERT}{large} SQuAD QA model and reduced to block level following  Eq.~\ref{equ:sentence_attention}~\citep{clark2019does}.
That is, attention from a block is averaged and attention to a block is accumulated.
By doing so, the attention from block [a,b] attending to block [c,d] is aggregated to one value.
% Attention values to a sentence are accumulated and attention values from a sentence is averaged.
% The attention weights related to this block, which contains attending to this block and attended by this block, are gathered and flattened as a feature vector for classification.
And the attention between a block and the question sentence, special tokens \texttt{"[CLS]"} and \texttt{"[SEP]"} are used to denote the attending relation of the block as a 6-dimensional vector.
Such vector from all attention heads in the layer are concatenated as the final classification feature for the corresponding block, which is 96-dimensional in the \model{Bert}{large} case.
With such block attention feature, simple logistic regression models are fitted to predict whether the answer exists within the range of the block.
As the attention weight value reflects the dependence of input positions, such feature is a good representation of the information processing behavior of Transformer layer.
% The result is shown in \Fig{fig:sentence_retrieval} with attention matrices from different layers.  
% As the figure suggesting, simple logistic regression with hand-crafted feature from attention weight achieves quite promising classification accuracy.
% This implies that the attending relationship between question and targets is indeed capable for figuring out answer position.
% This becomes our insight to utilize such attention information to narrow the possible answer position along with the processing of the input sequence.
% In the following section, we introduce our design to extract useful information from the attention weights for skimming decision.

\begin{equation} \label{equ:sentence_attention}
  \begin{split}
  BlockAttention&([a,b],[c,d]) =   \\ 
                                &    \frac{1}{b-a}\sum_{i=a}^b{\sum_{j=c}^d{Attention(i,j)}}
  \end{split}
\end{equation}
