# Supplementary material for: Block-Skim: Efficient Question Answering for Transformer
Source: arXiv:2112.08560 source file (2022-05-15)
Supplement: Supplementary file 3 [file appendix.tex]

\section{Training Loss}
We demonstrate the training loss optimization process with \model{BERT}{base} model on HotpotQA dataset.
The loss is logged every 200 updates.
As shown in \Fig{fig:loss}, the regularization of \ours{} objective on attention mechanism doesn't reduce the optimization speed.
Because we are not actually skimming blocks during training.

\begin{figure}[H]
  \centering
  \includegraphics[width=0.8\linewidth]{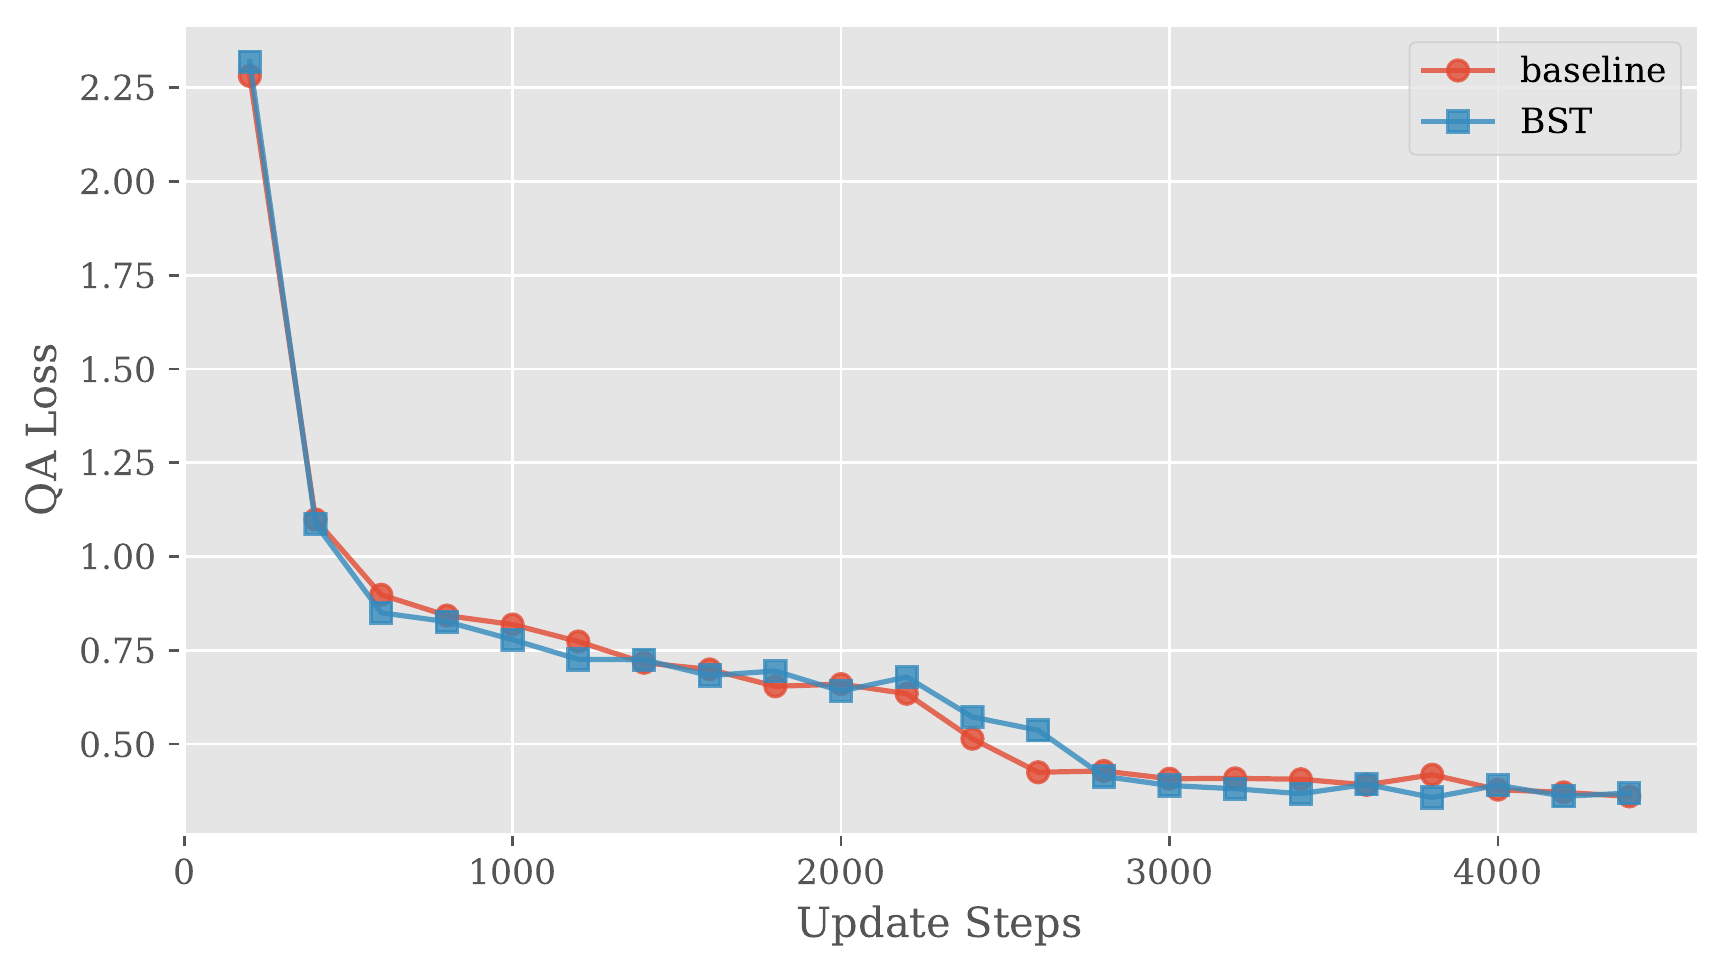}
  \caption{Training loss optimization process of vanilla \model{BERT}{base} and \model{BERT}{base} with \ours{} augmented.}
  \label{fig:loss}
\end{figure}

\section{\ours{} Classifier F1 Score}
Because we only show the \ours{} classifier accuracy performance of few layers in the main text for conciseness.
Here we present the F1 score results of \model{BERT}{base} and \model{BERT}{large} results of all layers as \Fig{fig:classifier}.
As expected, the augmented \ours{} classifiers have better prediction F1 scores at deeper layers.
This is because the deeper Transformer layers are more confident about the answer position and the attention weights are more informative.
As such, the \ours{} classifier manages to find the irrelevant blocks with higher accuracy.

\begin{figure}[H]
  \centering
  \includegraphics[width=0.8\linewidth]{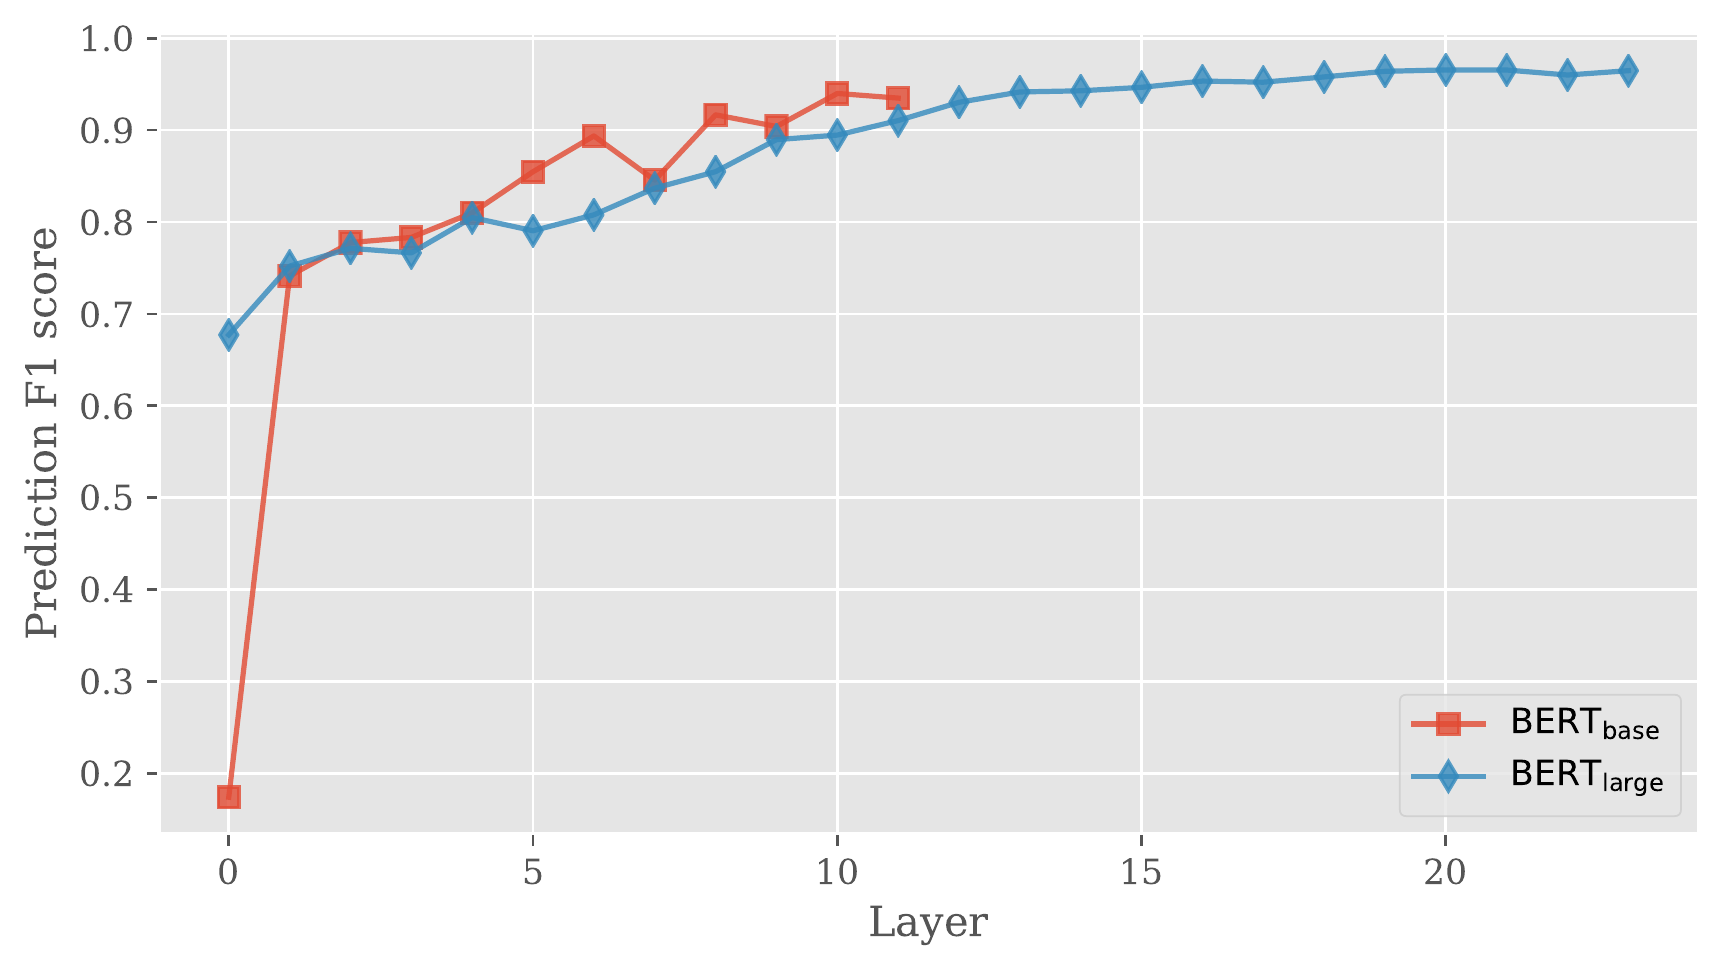}
  \caption{\ours{} classifier F1 score of each layer of \model{BERT}{base} and \model{model}{large} on SQuAD dataset.}
  \label{fig:classifier}
\end{figure}

% \fixme{rejection classifier f1 figure}

% \fixme{training loss figure}
