# Supplementary material for: Block-Skim: Efficient Question Answering for Transformer
Source: arXiv:2112.08560 source file (2022-05-15)
Supplement: Supplementary file 5 [file longtail.tex]

\section{Input Length Breakdown}

\begin{figure*}[t]
  \strut\newline
    \centering
    \includegraphics[width=\linewidth]{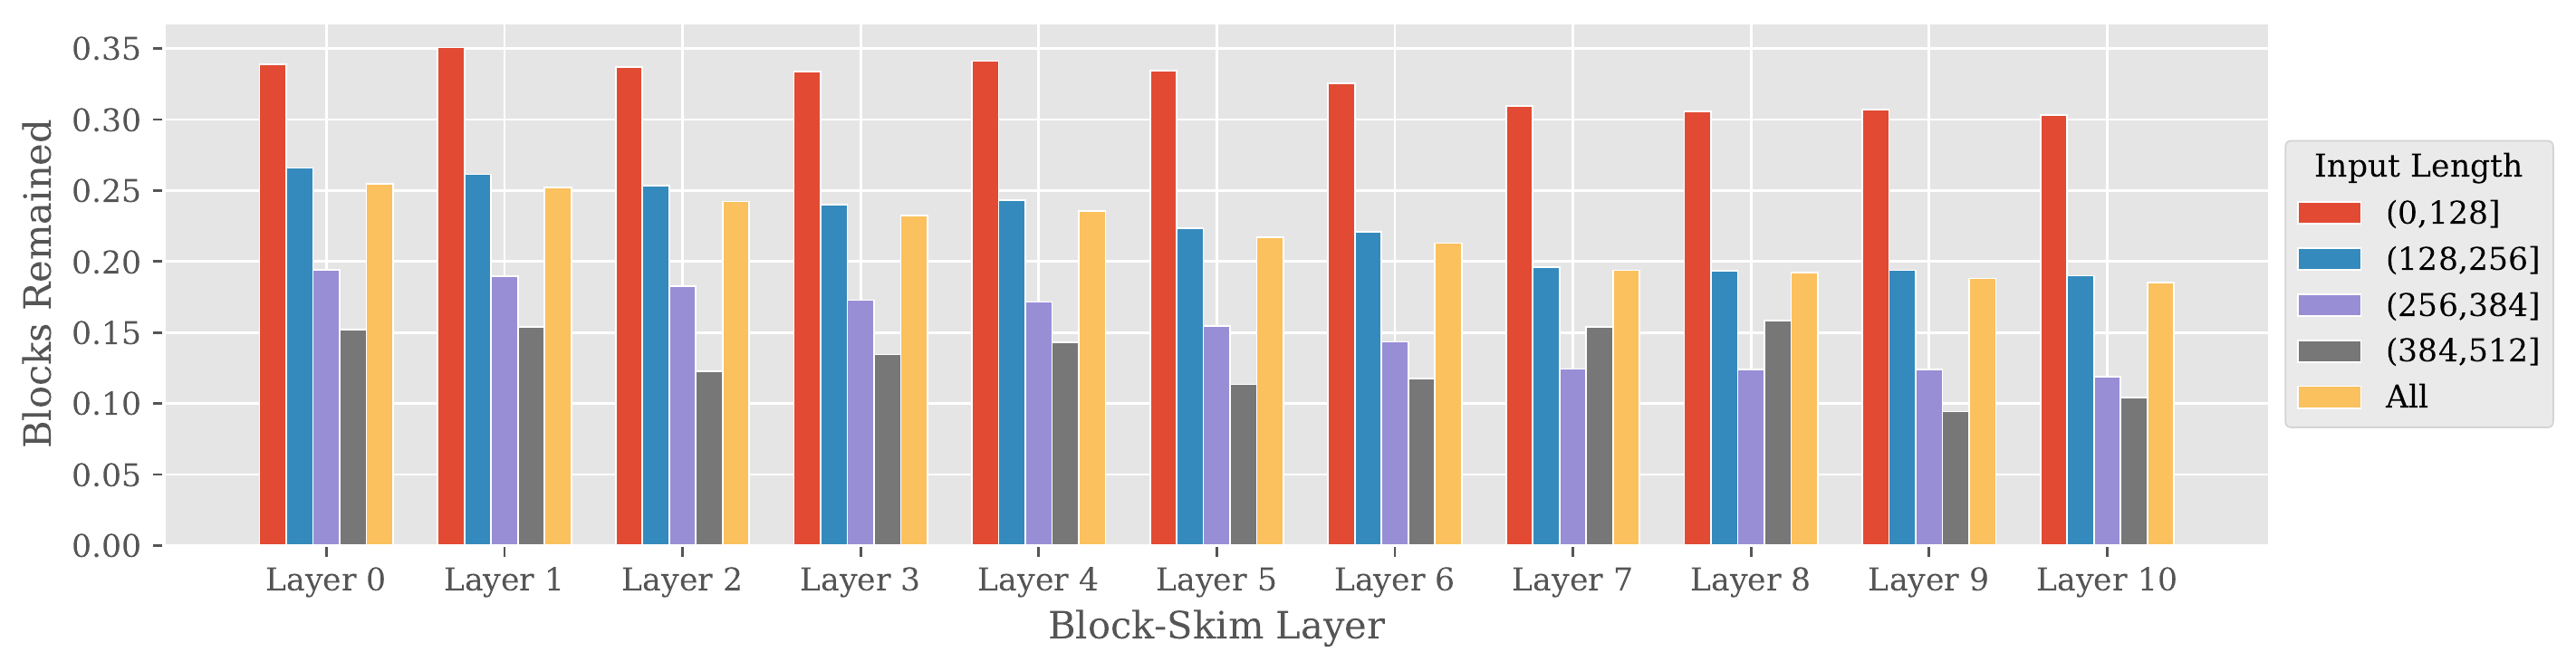}
    \caption{Breakdown of remained blocks numbers referring to input sequence length.}
\end{figure*}

Because we only show the \ours{} classifier skimming percentage of a few layers in the main text for conciseness.
We present the results of all layers here.
The result and conclusion are consistent with our demonstration in \Sec{sec:speedup}.
